# Supplementary material for: Structural Operational Semantics for Control Flow Graph Machines
Source: arXiv:1805.05400 source file (2018-05-14)
Supplement: Supplementary file 1 [file appendix.tex]

\ottgrammartabular{
\ottM\ottinterrule
\ottsort\ottinterrule
}

\ottdefnsJop
\ottdefnsJtype
